# Supplementary material for: JDT3D: Addressing the Gaps in LiDAR-Based Tracking-by-Attention
Source: arXiv:2407.04926 source file (2024-07-15)
Supplement: Supplementary file 1 [file X_supplemental.tex]

\section{Supplemental Materials}
\subsection{Qualitative Results}
Based on \cref{fig:qual_results}, we see excellent tracking performance of JDT3D. Properly detected tracks can maintain excellent consistency, even through difficult scenarios like occlusion. The visualizations also show the model's ability to predict the future trajectories of tracks in the scene properly.

A video of the visualizations can be found at \href{https://youtu.be/yv9vrpCSqR8?si=Y3pK6todbxqUlUhV}{https://youtu.be/yv9vrpCSqR8?si=Y3pK6todbxqUlUhV}

\subsection{Full Results}
We include a full table of class-specific metrics on both the nuScenes test and validation sets in \cref{tab:supp-jdt3d-test-all} and \cref{tab:supp-jdt3d-val-all}, respectively.

\begin{figure}
    \centering
    \includegraphics[width=0.75\linewidth]{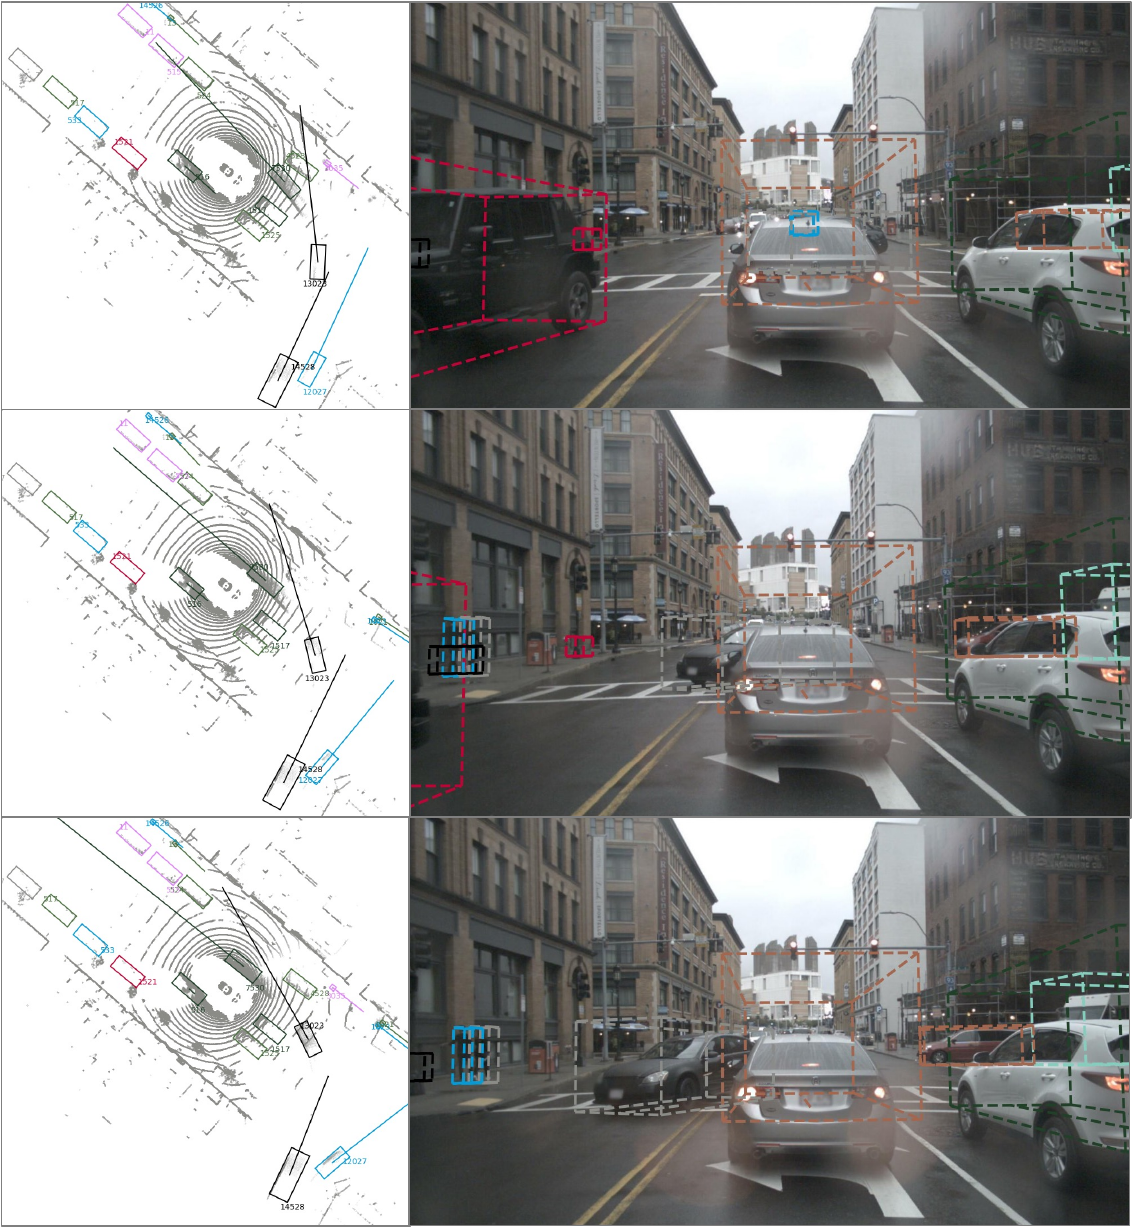}
    \caption{Qualitative results of JDT3D on a scene (consecutive frames from top to bottom) from nuScenes test set. For visual understanding, we show 3D bounding boxes projected into the BEV point cloud and the centre front camera image. Each bounding box has a unique track ID and is coloured accordingly. Line segments represent predicted future trajectories.}
    \label{fig:qual_results}
\end{figure}

\begin{landscape}
\begin{table}
\centering
\caption{Full results by class for JDT3D evaluated on the nuScenes test set.}
\begin{tabular}{l|cccccccccccccccc}
\specialrule{1pt}{0pt}{0pt}
Class   & AMOTA & AMOTP & RECALL & MOTAR & MOTA  & MOTP  & MT   & ML  & FAF  & TP    & FP   & FN    & IDS & FRAG & TID  & LGD  \\ \hline
Bicycle & 0.262 & 1.104 & 0.321  & 0.675 & 0.217 & 0.222 & 43   & 124 & 16.3 & 702   & 228  & 1484  & 0   & 3    & 0.68 & 0.80 \\
Bus     & 0.674 & 0.755 & 0.636  & 0.909 & 0.578 & 0.363 & 56   & 35  & 7.1  & 1082  & 99   & 619   & 0   & 1    & 0.64 & 0.71 \\
Car     & 0.751 & 0.613 & 0.795  & 0.901 & 0.714 & 0.255 & 2957 & 845 & 92.3 & 54352 & 5403 & 14042 & 124 & 210  & 0.60 & 1.00 \\
Motorcycle & 0.495 & 0.800 & 0.456  & 0.885 & 0.403 & 0.228 & 47   & 98  & 8.3  & 886   & 102  & 1058  & 1   & 3    & 0.56 & 0.80 \\
Pedestrian & 0.715 & 0.702 & 0.753  & 0.867 & 0.650 & 0.318 & 1284 & 449 & 66.4 & 25474 & 3379 & 8409  & 127 & 151  & 0.65 & 1.03 \\
Trailer & 0.616 & 0.906 & 0.631  & 0.810 & 0.511 & 0.507 & 77   & 57  & 27.4 & 1619  & 308  & 947   & 0   & 11   & 1.15 & 1.41 \\
Truck   & 0.504 & 0.979 & 0.611  & 0.691 & 0.422 & 0.351 & 210  & 183 & 39.9 & 5277  & 1633 & 3360  & 2   & 8    & 1.16 & 1.69 \\
\bottomrule
\end{tabular}
\label{tab:supp-jdt3d-test-all}
\end{table}
\end{landscape}

\begin{landscape}
\begin{table}
\centering
\caption{Full results by class for JDT3D evaluated on the nuScenes validation set.}
\begin{tabular}{l|cccccccccccccccc}
\specialrule{1pt}{0pt}{0pt}
Class   & AMOTA  & AMOTP  & Recall & MOTAR  & MOTA   & MOTP   & MT  & ML  & FAF   & TP   & FP   & FN   & IDS & FRAG & TID    & LGD   \\ \hline
Bicycle    & 0.3981 & 0.860  & 0.4711 & 0.6876 & 0.3236 & 0.1813 & 46  & 92  & 18.6  & 938  & 293  & 1054 & 1   & 1    & 1.285  & 1.354 \\
Bus        & 0.8117 & 0.6328 & 0.8229 & 0.9216 & 0.7571 & 0.4113 & 75  & 17  & 8.5   & 1735 & 136  & 374  & 3   & 14   & 0.5652 & 1.114 \\
Car        & 0.7827 & 0.5686 & 0.7944 & 0.9308 & 0.7386 & 0.2514 & 2361 & 746 & 55.76 & 46276 & 3204 & 11992 & 49 & 106 & 0.5708 & 0.8826 \\
Motorcycle & 0.6376 & 0.6847 & 0.6657 & 0.7673 & 0.5104 & 0.2857 & 66  & 46  & 20.21 & 1315 & 306  & 661  & 1   & 2    & 1.201  & 1.316 \\
Pedestrian & 0.7357 & 0.6806 & 0.7763 & 0.862  & 0.6662 & 0.3296 & 1044 & 373 & 59.47 & 19649 & 2712 & 5688  & 86 & 90  & 0.6434 & 0.9963 \\
Trailer    & 0.4511 & 1.124  & 0.4969 & 0.7535 & 0.3744 & 0.5834 & 51  & 74  & 26.88 & 1205 & 297  & 1220 & 0   & 8    & 0.7623 & 1.287 \\
Truck      & 0.5321 & 0.9763 & 0.6556 & 0.7204 & 0.4716 & 0.3652 & 252 & 166 & 46.09 & 6317 & 1766 & 3323 & 10  & 25   & 1.066  & 1.763 \\
\bottomrule
\end{tabular}
\label{tab:supp-jdt3d-val-all}
\end{table}
\end{landscape}
